# Supplementary material for: Relativistic Two-component Double Ionization Potential Equation-of-Motion Coupled Cluster with the Dirac--Coulomb--Breit Hamiltonian
Source: arXiv:2505.00499 ancillary file (2025-07-25)
Supplement: Supplementary file 1 [file x2c_dip_eom_cc_si.pdf]

# Supporting Information for: Relativistic Two-component Double Ionization Potential Equation-of-Motion Coupled Cluster with the Dirac–Coulomb–Breit Hamiltonian

Run R. Li,[1] Stephen H. Yuwono,[1] Marcus D. Liebenthal,[1] Tianyuan Zhang,[2] Xiaosong Li,[2] and A. Eugene DePrince III[1, a)]

[1)] *Department of Chemistry and Biochemistry, Florida State University, Tallahassee, FL 32306-4390*

[2)] *Department of Chemistry, University of Washington, Seattle, WA 98195, USA*

TABLE S1. Double ionization potentials (eV) calculated using DCB-X2C-DIP-EOMCCSD within the ANO-RCC-VTZP basis sets. All-electron calculations are compared to those in which only electrons in the valence shell plus one inner shell are correlated.

| | State | full space | frozen core | difference |
|---|---|---|---|---|
| Ar | $^3P_2$ | 43.316 | 43.316 | 0.000 |
| | $^3P_1$ | 43.455 | 43.455 | 0.000 |
| | $^3P_0$ | 43.514 | 43.514 | 0.000 |
| | $^1D_2$ | 45.107 | 45.107 | 0.000 |
| | $^1S_0$ | 47.574 | 47.574 | 0.000 |
| Kr | $^3P_2$ | 38.045 | 38.046 | 0.001 |
| | $^3P_1$ | 38.595 | 38.596 | 0.001 |
| | $^3P_0$ | 38.695 | 38.697 | 0.001 |
| | $^1D_2$ | 39.906 | 39.907 | 0.001 |
| | $^1S_0$ | 42.250 | 42.251 | 0.001 |
| Xe | $^3P_2$ | 32.942 | 32.949 | 0.007 |
| | $^3P_0$ | 33.952 | 33.959 | 0.007 |
| | $^3P_1$ | 34.109 | 34.115 | 0.006 |
| | $^1D_2$ | 35.056 | 35.062 | 0.006 |
| | $^1S_0$ | 37.427 | 37.433 | 0.006 |
| $Cl_2$ | $^3\Sigma^-$ | 31.288 | 31.288 | 0.000 |
| | $^1\Delta$ | 31.798 | 31.798 | 0.000 |
| | $^1\Sigma^+$ | 32.189 | 32.189 | 0.000 |
| | $^1\Sigma^-$ | 33.215 | 33.215 | 0.000 |
| $Br_2$ | $^3\Sigma^-_{g0}$ | 28.233 | 28.234 | 0.001 |
| | $^3\Sigma^-_{g1}$ | 28.375 | 28.376 | 0.001 |
| | $^1\Delta_{g2}$ | 28.793 | 28.794 | 0.001 |
| | $^1\Sigma^+_{g0}$ | 29.258 | 29.259 | 0.001 |
| HBr | $^3\Sigma^-$ | 32.614 | 32.614 | 0.001 |
| | $^1\Delta$ | 33.997 | 33.998 | 0.001 |
| | $^1\Sigma^+$ | 35.290 | 35.291 | 0.001 |
| HI | $^3\Sigma^-_0$ | 29.052 | 29.058 | 0.006 |
| | $^1\Sigma^-_1$ | 29.267 | 29.272 | 0.005 |
| | $^1\Delta$ | 30.323 | 30.328 | 0.005 |
| | $^1\Sigma^+$ | 31.620 | 31.625 | 0.005 |

[a)] Electronic mail: adeprince@fsu.edu

TABLE S2. Double ionization potentials (eV) calculated using 1eX2C- and DCB-X2C-DIP-EOMCCSD within the ANO-RCC-V$n$ZP ($n$ = D, T, Q) basis sets. Only electrons in the valence shell plus one inner shell are correlated.

| | State | ANO-RCC-VDZP | | | ANO-RCC-VTZP | | | ANO-RCC-VQZP | | |
|---|---|---|---|---|---|---|---|---|---|---|
| | | 1eX2C | mmfX2C | absolute difference | 1eX2C | mmfX2C | absolute difference | 1eX2C | mmfX2C | absolute difference |
| Ar | $^3P_2$ | 42.775 | 42.945 | 0.170 | 43.292 | 43.316 | 0.024 | 43.615 | 43.610 | 0.006 |
| | $^3P_1$ | 42.905 | 43.081 | 0.177 | 43.424 | 43.455 | 0.032 | 43.754 | 43.749 | 0.004 |
| | $^3P_0$ | 42.960 | 43.140 | 0.180 | 43.479 | 43.514 | 0.034 | 43.811 | 43.807 | 0.004 |
| | $^1D_2$ | 44.721 | 44.894 | 0.173 | 45.079 | 45.107 | 0.028 | 45.363 | 45.358 | 0.005 |
| | $^1S_0$ | 46.973 | 47.147 | 0.174 | 47.546 | 47.574 | 0.028 | 47.811 | 47.805 | 0.005 |
| Kr | $^3P_2$ | 37.585 | 37.670 | 0.085 | 38.076 | 38.046 | 0.030 | 38.424 | 38.386 | 0.039 |
| | $^3P_1$ | 38.089 | 38.209 | 0.120 | 38.582 | 38.596 | 0.013 | 38.959 | 38.939 | 0.020 |
| | $^3P_0$ | 38.189 | 38.306 | 0.117 | 38.686 | 38.697 | 0.010 | 39.061 | 39.039 | 0.021 |
| | $^1D_2$ | 39.571 | 39.682 | 0.110 | 39.904 | 39.907 | 0.004 | 40.232 | 40.208 | 0.024 |
| | $^1S_0$ | 41.687 | 41.807 | 0.120 | 42.237 | 42.251 | 0.014 | 42.551 | 42.532 | 0.019 |
| Xe | $^3P_2$ | 32.412 | 32.476 | 0.064 | 33.026 | 32.949 | 0.077 | 33.263 | 33.161 | 0.102 |
| | $^3P_0$ | 33.365 | 33.462 | 0.097 | 33.994 | 33.959 | 0.035 | 34.253 | 34.168 | 0.085 |
| | $^3P_1$ | 33.482 | 33.622 | 0.140 | 34.100 | 34.115 | 0.015 | 34.400 | 34.337 | 0.063 |
| | $^1D_2$ | 34.601 | 34.731 | 0.130 | 35.056 | 35.062 | 0.006 | 35.327 | 35.260 | 0.067 |
| | $^1S_0$ | 36.805 | 36.983 | 0.179 | 37.370 | 37.433 | 0.063 | 37.666 | 37.623 | 0.043 |
| $Cl_2$ | $^3\Sigma^-$ | 30.807 | 30.730 | 0.077 | 31.301 | 31.288 | 0.013 | 31.561 | 31.551 | 0.010 |
| | $^1\Delta$ | 31.344 | 31.266 | 0.078 | 31.810 | 31.798 | 0.013 | 32.061 | 32.050 | 0.010 |
| | $^1\Sigma^+$ | 31.695 | 31.617 | 0.078 | 32.201 | 32.189 | 0.012 | 32.450 | 32.440 | 0.010 |
| | $^1\Sigma^-$ | 32.728 | 32.639 | 0.089 | 33.235 | 33.215 | 0.019 | 33.493 | 33.480 | 0.013 |
| $Br_2$ | $^3\Sigma^-_{g0}$ | 27.806 | 27.705 | 0.101 | 28.270 | 28.234 | 0.036 | 28.560 | 28.525 | 0.035 |
| | $^3\Sigma^-_{g1}$ | 27.930 | 27.845 | 0.085 | 28.396 | 28.376 | 0.020 | 28.694 | 28.671 | 0.023 |
| | $^1\Delta_{g2}$ | 28.380 | 28.294 | 0.087 | 28.814 | 28.794 | 0.020 | 29.101 | 29.077 | 0.023 |
| | $^1\Sigma^+_{g0}$ | 28.794 | 28.722 | 0.072 | 29.263 | 29.259 | 0.004 | 29.556 | 29.545 | 0.011 |
| HBr | $^3\Sigma^-$ | 32.087 | 32.054 | 0.033 | 32.643 | 32.614 | 0.028 | 32.916 | 32.890 | 0.026 |
| | $^1\Delta$ | 33.656 | 33.626 | 0.030 | 34.021 | 33.998 | 0.024 | 34.263 | 34.241 | 0.022 |
| | $^1\Sigma^+$ | 34.859 | 34.831 | 0.028 | 35.309 | 35.291 | 0.018 | 35.548 | 35.530 | 0.018 |
| HI | $^3\Sigma^-_0$ | 28.433 | 28.341 | 0.092 | 29.157 | 29.058 | 0.100 | 29.379 | 29.289 | 0.090 |
| | $^1\Sigma^-_1$ | 28.616 | 28.540 | 0.075 | 29.347 | 29.272 | 0.075 | 29.581 | 29.506 | 0.075 |
| | $^1\Delta$ | 29.875 | 29.790 | 0.085 | 30.408 | 30.328 | 0.080 | 30.616 | 30.537 | 0.078 |
| | $^1\Sigma^+$ | 31.112 | 31.034 | 0.078 | 31.684 | 31.625 | 0.059 | 31.896 | 31.830 | 0.066 |

TABLE S3. Excitation energies (eV) of doubly ionized states calculated using 1eX2C- and DCB-X2C-DIP-EOMCCSD within the ANO-RCC-V*n*ZP (*n* = D, T, Q) basis sets. Only electrons in the valence shell plus one inner shell are correlated.

| | State | ANO-RCC-VDZP | | | ANO-RCC-VTZP | | | ANO-RCC-VQZP | | |
|---|---|---|---|---|---|---|---|---|---|---|
| | | 1eX2C | mmfX2C | absolute difference | 1eX2C | mmfX2C | absolute difference | 1eX2C | mmfX2C | absolute difference |
| Ar | $^3P_1$ | 0.131 | 0.137 | 0.007 | 0.132 | 0.140 | 0.008 | 0.138 | 0.140 | 0.001 |
| | $^3P_0$ | 0.186 | 0.195 | 0.009 | 0.187 | 0.198 | 0.011 | 0.196 | 0.198 | 0.002 |
| | $^1D_2$ | 1.946 | 1.949 | 0.003 | 1.787 | 1.791 | 0.004 | 1.748 | 1.748 | 0.001 |
| | $^1S_0$ | 4.198 | 4.202 | 0.003 | 4.254 | 4.258 | 0.005 | 4.195 | 4.196 | 0.001 |
| Kr | $^3P_1$ | 0.504 | 0.539 | 0.035 | 0.506 | 0.549 | 0.043 | 0.535 | 0.554 | 0.019 |
| | $^3P_0$ | 0.603 | 0.636 | 0.032 | 0.610 | 0.650 | 0.040 | 0.636 | 0.654 | 0.017 |
| | $^1D_2$ | 1.986 | 2.011 | 0.025 | 1.827 | 1.861 | 0.033 | 1.807 | 1.822 | 0.014 |
| | $^1S_0$ | 4.102 | 4.137 | 0.035 | 4.161 | 4.205 | 0.044 | 4.127 | 4.146 | 0.019 |
| Xe | $^3P_0$ | 0.953 | 0.986 | 0.033 | 0.968 | 1.010 | 0.042 | 0.990 | 1.007 | 0.017 |
| | $^3P_1$ | 1.070 | 1.146 | 0.076 | 1.074 | 1.166 | 0.092 | 1.137 | 1.176 | 0.039 |
| | $^1D_2$ | 2.188 | 2.255 | 0.067 | 2.030 | 2.113 | 0.083 | 2.064 | 2.099 | 0.035 |
| | $^1S_0$ | 4.392 | 4.507 | 0.115 | 4.344 | 4.484 | 0.140 | 4.403 | 4.462 | 0.059 |
| $Cl_2$ | $^1\Delta$ | 0.537 | 0.536 | 0.001 | 0.510 | 0.510 | 0.000 | 0.499 | 0.499 | 0.000 |
| | $^1\Sigma^+$ | 0.888 | 0.887 | 0.001 | 0.900 | 0.901 | 0.001 | 0.888 | 0.889 | 0.001 |
| | $^1\Sigma^-$ | 1.921 | 1.909 | 0.012 | 1.934 | 1.928 | 0.006 | 1.932 | 1.929 | 0.002 |
| $Br_2$ | $^3\Sigma^-_{g1}$ | 0.124 | 0.139 | 0.016 | 0.126 | 0.142 | 0.017 | 0.134 | 0.146 | 0.012 |
| | $^1\Delta_{g2}$ | 0.574 | 0.588 | 0.014 | 0.544 | 0.560 | 0.016 | 0.541 | 0.552 | 0.012 |
| | $^1\Sigma^+_{g0}$ | 0.988 | 1.017 | 0.029 | 0.993 | 1.025 | 0.032 | 0.996 | 1.020 | 0.024 |
| HBr | $^1\Delta$ | 1.569 | 1.572 | 0.003 | 1.379 | 1.383 | 0.005 | 1.347 | 1.350 | 0.003 |
| | $^1\Sigma^+$ | 2.772 | 2.777 | 0.005 | 2.666 | 2.676 | 0.010 | 2.632 | 2.640 | 0.007 |
| HI | $^1\Sigma^-_1$ | 0.183 | 0.200 | 0.017 | 0.190 | 0.214 | 0.025 | 0.202 | 0.217 | 0.015 |
| | $^1\Delta$ | 1.442 | 1.450 | 0.008 | 1.251 | 1.271 | 0.020 | 1.237 | 1.248 | 0.011 |
| | $^1\Sigma^+$ | 2.679 | 2.693 | 0.015 | 2.527 | 2.567 | 0.041 | 2.517 | 2.541 | 0.024 |

TABLE S4. Excitation energies (eV) of doubly ionized states calculated using DCB-X2C-DIP-EOMCCSD within the ANO-RCC-V*n*ZP (*n* = D, T, Q), x2c-SVPall-2c, x2c-VTZPP-all-2c, and dyall.acv*nz* basis sets. Only electrons in the valence shell plus one inner shell are correlated.

| | State | experiment | ANO-RCC-V*n*ZP | | | | x2c | | dyall.acv*nz* | |
|---|---|---|---|---|---|---|---|---|---|---|
| | | | D | T | Q | full | SVPall-2c | TZVPPall-2c | D | T |
| Ar | $^3P_2$ | 43.389[a] | 42.945 | 43.316 | 43.610 | 43.696 | 42.564 | 43.296 | 43.121 | 43.520 |
| | $^3P_1$ | 43.527 | 43.083 | 43.455 | 43.749 | 43.836 | 42.704 | 43.435 | 43.260 | 43.662 |
| | $^3P_0$ | 43.584 | 43.140 | 43.514 | 43.807 | 43.895 | 42.762 | 43.494 | 43.318 | 43.721 |
| | $^1D_2$ | 45.126 | 44.894 | 45.107 | 45.358 | 45.439 | 44.490 | 45.096 | 45.051 | 45.299 |
| | $^1S_0$ | 47.514 | 47.147 | 47.574 | 47.805 | 47.893 | 46.680 | 47.559 | 47.327 | 47.756 |
| Kr | $^3P_2$ | 38.359[a] | 37.670 | 38.046 | 38.386 | 38.484 | 37.583 | 38.073 | 38.037 | 38.327 |
| | $^3P_1$ | 38.923 | 38.209 | 38.596 | 38.939 | 39.047 | 38.135 | 38.630 | 38.605 | 38.902 |
| | $^3P_0$ | 39.018 | 38.306 | 38.697 | 39.039 | 39.145 | 38.232 | 38.731 | 38.702 | 39.001 |
| | $^1D_2$ | 40.175 | 39.682 | 39.907 | 40.208 | 40.308 | 39.595 | 39.950 | 40.024 | 40.193 |
| | $^1S_0$ | 42.461 | 41.807 | 42.251 | 42.532 | 42.634 | 41.731 | 42.285 | 42.215 | 42.537 |
| Xe | $^3P_2$ | 33.105[a] | 32.476 | 32.949 | 33.161 | 33.240 | 32.266 | 32.822 | 32.698 | 33.019 |
| | $^3P_0$ | 34.113 | 33.462 | 33.959 | 34.168 | 34.252 | 33.235 | 33.857 | 33.720 | 34.059 |
| | $^3P_1$ | 34.319 | 33.622 | 34.115 | 34.337 | 34.429 | 33.423 | 34.036 | 33.910 | 34.250 |
| | $^1D_2$ | 35.225 | 34.731 | 35.062 | 35.260 | 35.348 | 34.563 | 35.031 | 35.005 | 35.205 |
| | $^1S_0$ | 37.581 | 36.983 | 37.433 | 37.623 | 37.719 | 36.671 | 37.450 | 37.293 | 37.629 |
| $Cl_2$ | $^3\Sigma^-$ | 31.13[b] | 30.730 | 31.288 | 31.551 | 31.648 | 30.806 | 31.296 | 31.147 | 31.521 |
| | $^1\Delta$ | 31.74 | 31.266 | 31.798 | 32.050 | 32.144 | 31.346 | 31.806 | 31.687 | 32.025 |
| | $^1\Sigma^+$ | 32.12 | 31.617 | 32.189 | 32.440 | 32.533 | 31.696 | 32.195 | 32.047 | 32.413 |
| | $^1\Sigma^-$ | 32.97 | 32.639 | 33.215 | 33.480 | 33.570 | 32.734 | 33.212 | 33.075 | 33.433 |
| $Br_2$ | $^3\Sigma^-_{g0}$ | 28.39[c] | 27.705 | 28.234 | 28.525 | 28.639 | 27.857 | 28.248 | 28.269 | 28.527 |
| | $^3\Sigma^-_{g1}$ | 28.53 | 27.845 | 28.376 | 28.671 | 28.789 | 28.003 | 28.394 | 28.423 | 28.683 |
| | $^1\Delta_{g2}$ | 28.91 | 28.294 | 28.794 | 29.077 | 29.191 | 28.456 | 28.812 | 28.861 | 29.090 |
| | $^1\Sigma^+_{g0}$ | 29.38 | 28.722 | 29.259 | 29.545 | 29.661 | 28.896 | 29.279 | 29.314 | 29.563 |
| HBr | $^3\Sigma^-$ | 32.62[d] | 32.054 | 32.614 | 32.890 | 33.003 | 32.006 | 32.627 | 32.505 | 32.910 |
| | $^1\Delta$ | 33.95 | 33.626 | 33.998 | 34.241 | 34.348 | 33.568 | 34.027 | 34.025 | 34.283 |
| | $^1\Sigma^+$ | 35.19 | 34.831 | 35.291 | 35.530 | 35.637 | 34.781 | 35.317 | 35.262 | 35.578 |
| HI | $^3\Sigma^-_0$ | 29.15[e] | 28.341 | 29.058 | 29.289 | 29.357 | 28.229 | 28.976 | 28.760 | 29.204 |
| | $^1\Sigma^-_1$ | 29.37 | 28.540 | 29.272 | 29.506 | 29.580 | 28.438 | 29.197 | 28.983 | 29.435 |
| | $^1\Delta$ | 30.39 | 29.790 | 30.328 | 30.537 | 30.608 | 29.716 | 30.301 | 30.211 | 30.499 |
| | $^1\Sigma^+$ | 31.64 | 31.034 | 31.625 | 31.830 | 31.906 | 30.898 | 31.612 | 31.468 | 31.814 |

[a] A. Kramida, Yu. Ralchenko, J. Reader, and and NIST ASD Team, NIST Atomic Spectra Database (ver. 5.12), [Online]. Available: https://physics.nist.gov/asd [2025, March 18]. National Institute of Standards and Technology, Gaithersburg, MD. (2024).

[b] A. G. McConkey, G. Dawber, L. Avaldi, M. A. MacDonald, G. C. King, and R. I. Hall, "Threshold photoelectrons coincidence spectroscopy of doubly charged ions of hydrogen chloride and chlorine," Journal of Physics B: Atomic, Molecular and Optical Physics 27, 271 (1994).

[c] T. Fleig, D. Edvardsson, S. T. Banks, and J. H. Eland, "A theoretical and experimental study of the double photoionisation of molecular bromine and a new double ionisation mechanism," Chemical Physics 343, 270–280 (2008), theoretical Spectroscopy and its Impact on Experiment.

[d] J. H. Eland, "Complete double photoionisation spectra of small molecules from tof-pepeco measurements," Chemical Physics 294, 171–186 (2003).

[e] A. J. Yencha, A. M. Juarez, S. Pui Lee, G. C. King, F. R. Bennett, F. Kemp, and I. R. McNab, "Photo-double ionization of hydrogen iodide: experi- ment and theory," Chemical Physics 303, 179–187 (2004).

TABLE S5. Excitation energies (eV) of doubly ionized states calculated using non-relativistic DIP-EOMCCSD(4$h$2$p$) and DIP-EOMCCSDT within the ANO-RCC-VDZP and ANO-RCC-VTZP basis sets for Ar, Kr, and Xe. Only electrons in the valence shell plus one inner shell are correlated.

| | State | DIP-EOMCCSD(4$h$2$p$) | DIP-EOMCCSDT | |
|---|---|---|---|---|
| | | ANO-RCC-VDZP | ANO-RCC-VDZP | ANO-RCC-VTZP |
| Ar | $^3P_2$ | 42.596 | 42.638 | 42.876 |
| | $^3P_1$ | 42.731 | 42.773 | 43.011 |
| | $^3P_0$ | 42.787 | 42.829 | 43.068 |
| | $^1D_2$ | 44.545 | 44.585 | 44.687 |
| | $^1S_0$ | 46.823 | 46.858 | 47.127 |
| Kr | $^3P_2$ | 37.493 | 37.509 | 37.778 |
| | $^3P_1$ | 38.022 | 38.038 | 38.313 |
| | $^3P_0$ | 38.120 | 38.136 | 38.415 |
| | $^1D_2$ | 39.506 | 39.521 | 39.651 |
| | $^1S_0$ | 41.667 | 41.677 | 41.995 |
| Xe | $^3P_2$ | —[a] | 32.357 | —[b] |
| | $^3P_0$ | —[a] | 33.332 | —[b] |
| | $^3P_1$ | —[a] | 33.493 | —[b] |
| | $^1D_2$ | —[a] | 34.593 | —[b] |
| | $^1S_0$ | —[a] | 36.830 | —[b] |

[a] Not fully converged. These DIP values are ∼0.01–0.04 eV lower compared to those resulting from DIP-EOMCCSDT/ANO-RCC-VDZP calculations at the same residual convergence.
[b] Calculations not performed.

TABLE S6. Excitation energies (eV) of doubly ionized states calculated using non-relativistic DIP-EOMCCSD and DIP-EOMCCSDT within the ANO-RCC basis set family for Ar, Kr, and Xe. Only electrons in the valence shell plus one inner shell are correlated.

| | State | DIP-EOMCCSD/ANO-RCC-V$n$ZP | | | | DIP-EOMCCSDT/ANO-RCC-V$n$ZP | | | |
|---|---|---|---|---|---|---|---|---|---|
| | | $n$ =D | $n$ =T | $n$ =Q | full | $n$ =D | $n$ =T | $n$ =Q | full |
| Ar | $^3P_{2,1,0}$ | 42.910 | 43.378 | 43.731 | 43.825 | 42.602 | 42.936 | 43.282 | 43.337 |
| | $^1D_2$ | 44.781 | 45.091 | 45.402 | 45.490 | 44.472 | 44.670 | 44.972 | 45.019 |
| | $^1S_0$ | 47.013 | 47.541 | 47.833 | 47.929 | 46.724 | 47.093 | 47.369 | 47.414 |
| Kr | $^3P_{2,1,0}$ | 37.497 | 38.448 | 38.895 | 38.972 | 37.508 | 38.169 | 38.593 | 38.618 |
| | $^1D_2$ | 39.207 | 39.926 | 40.332 | 40.403 | 39.243 | 39.667 | 40.050 | 40.068 |
| | $^1S_0$ | 40.753 | 42.128 | 42.518 | 42.595 | 40.790 | 41.869 | 42.226 | 42.245 |
| Xe | $^3P_{2,0,1}$ | 35.065 | 34.496 | 35.161 | 34.900 | 35.112 | 34.161 | 34.752 | —[a] |
| | $^1D_2$ | 36.494 | 35.666 | 36.303 | 36.036 | 36.551 | 35.327 | 35.897 | —[a] |
| | $^1S_0$ | 37.233 | 37.255 | 37.923 | 37.739 | 37.295 | 36.880 | 37.492 | —[a] |

[a] Calculations not performed.

TABLE S7. Possible routes to obtain corrections to double IP energies (eV), using relativistic and non-relativitic DIP-EOMCCSD and DIP-EOMCCSDT in the ANO-RCC family basis set.

| Correction | Ar | Kr | Xe |
|---|---|---|---|
| Average correction by basis set level (DZ) | | | |
| NR/SD/DZ → NR/SD/TZ | 0.448 | 0.893 | -0.502 |
| NR/SDT/DZ → NR/SDT/TZ | 0.314 | 0.602 | -0.899 |
| DCB/SD/DZ → DCB/SD/TZ | 0.352 | 0.345 | 0.449 |
| DCB/SDT/DZ → DCB/SDT/TZ | 0.217 | 0.238 | —[a] |
| Average correction by basis set level (TZ) | | | |
| NR/SD/TZ → NR/SD/QZ | 0.332 | 0.437 | 0.660 |
| NR/SDT/TZ → NR/SDT/QZ | 0.323 | 0.413 | 0.591 |
| DCB/SD/TZ → DCB/SD/QZ | 0.273 | 0.331 | 0.206 |
| Average correction by basis set level (QZ) | | | |
| NR/SD/QZ → NR/SD/full | 0.093 | 0.076 | -0.247 |
| NR/SDT/QZ → NR/SDT/full | 0.051 | 0.023 | —[a] |
| DCB/SD/QZ → DCB/SD/full | 0.086 | 0.103 | 0.088 |
| Average correction by correlation level (DZ) | | | |
| NR/SD/DZ → NR/SDT/DZ | -0.304 | 0.018 | 0.053 |
| DCB/SD/DZ → DCB/SDT/DZ | -0.305 | -0.166 | -0.134 |
| Average correction by correlation level (TZ) | | | |
| NR/SD/TZ → NR/SDT/TZ | -0.439 | -0.274 | -0.344 |
| DCB/SD/TZ → DCB/SDT/TZ | -0.439 | -0.272 | —[a] |
| Average correction by both correlation and basis set level (DZ) | | | |
| NR/SD/DZ → NR/SDT/TZ | 0.009 | 0.619 | -0.846 |
| DCB/SD/DZ → DCB/SDT/TZ | -0.088 | 0.072 | —[a] |
| Average correction by relativistic effect (DZ) | | | |
| NR/SD/DZ → DCB/SD/DZ | 0.137 | 0.543 | -1.529 |
| NR/SDT/DZ → DCB/SDT/DZ | 0.136 | 0.359 | -1.715 |
| Average correction by relativistic effect (TZ) | | | |
| NR/SD/TZ → DCB/SD/TZ | 0.040 | -0.006 | -0.578 |
| NR/SDT/TZ → DCB/SDT/TZ | 0.039 | -0.004 | —[a] |
| Average correction by both relativistic effect and basis set (DZ) | | | |
| NR/SD/DZ → DCB/SD/TZ | 0.488 | 0.887 | -1.080 |
| NR/SDT/DZ → DCB/SDT/TZ | 0.353 | 0.597 | —[a] |

[a] DCB/SDT/TZ and NR/SDT/full not performed for Xe due to computational cost.
